# Supplementary material for: Viscoelastic multiscaling in immersed networks
Source: arXiv:2004.02271 source file (2020-04-05)
Supplement: Supplementary file 1 [file main_SM.pdf]

# Supplementary material:
# Viscoelastic multiscaling in immersed networks

J. L. B. de Araújo, J. S. de Sousa, W. P. Ferreira, and C. L. N. Oliveira
*Departamento de Física, Universidade Federal do Ceará, 60451-970 Fortaleza, Ceará, Brazil*

## I. FORCE CURVES DETERMINATION

The indentation force curve, at a time $t$, is obtained by solving the following integral,

$$F(t) = \Omega(\beta) \int_0^t R(t-t') \frac{d\delta^\beta(t')}{dt'} dt', \tag{1}$$

where $\beta$ and $\Omega(\beta)$ are parameter related to the indenter geometry (see Table I), and $R(t)$ is the time-dependent relaxation function. During load stage, when the sample is pressed down by the indenter with constant velocity, $F$ increases. After reaching the maximum indentation, the indenter stops and the sample relaxes due to its viscoelastic properties leading $F$ to decrease.

For a relaxation experiment, the load (l) and dwell (d) curves are given, respectively, by

$$f_l(t) = \int_0^t R(t-t') \frac{d\bar{\delta}_l^\beta(t')}{dt'} dt', \quad t \le \tau_l, \tag{2}$$

$$f_d(t) = \int_0^{\tau_l} R(t-t') \frac{d\bar{\delta}_l^\beta(t')}{dt'} dt' + \int_{\tau_l}^t R(t-t') \frac{d\bar{\delta}_d^\beta(t')}{dt'} dt', \quad t \ge \tau_l, \tag{3}$$

where $\tau_l$ is the loading time. The indentation history $\delta(t)$ is normalized by the maximum indentation $\delta_0$ achieved at $t = \tau_l$, such that $\bar{\delta}(t) = \delta(t)/\delta_0$, and the force at each stage is also normalized by geometric constants,

$$f(t) = F(t)/(\Omega(\beta)\delta_0^\beta). \tag{4}$$

In order to solve Eq. 1, we consider $R(t)$ from the so-called Standard Linear Solid model, given by

$$R(t) = E_\infty + E_0 e^{-t/\tau}, \tag{5}$$

where $\tau$ is the relaxation time, and $E_\infty$ and $E_0$ are elastic moduli.

The load $\delta_l(t)$ indentation profile is well described by a linear function in time, while the dwell profile $\delta_d(t)$ is represented by a smooth increasing function in time $g(t)$ (such that $dg/dt \approx 0$). More specifically, one can write

$$\delta_l(t) = \delta_0 \frac{t}{\tau_l}, \tag{6}$$

$$\delta_d(t) = \delta_0 [1 + g(t - \tau_l)], \tag{7}$$

such that the last term of Eq. (3) vanishes.

Replacing the equations (5) in (1), we obtain the behavior of force during the load and relaxation processes

$$f_l(t) = \int_0^t \left( E_\infty + E_0 e^{-(t-t')/\tau} \right) \frac{3}{2\tau_l^{3/2}} t'^{1/2} dt', \qquad t \le \tau_l, \tag{8}$$

$$f_d(t) = \int_0^{\tau_l} \left( E_\infty + E_0 e^{-(t-t')/\tau} \right) \frac{3}{2\tau_l^{3/2}} t'^{1/2} dt', \qquad t \ge \tau_l, \tag{9}$$

TABLE I: Dependence of the parameters $\beta$ and $\Omega(\beta)$ on the indenter geometry. Below, $\nu$ represents the Poisson ratio and $\delta$ is the indentation. We assume $\nu = 0.5$.

| Geometry | $\beta$ | $\Omega(\beta)$ | contact radius | Obs. |
|---|---|---|---|---|
| flat cylinder | 1.0 | $\frac{2R}{(1-\nu^2)}$ | $R$ | $R$ is the indenter radius |
| spherical | 1.5 | $\frac{4}{3}\frac{\sqrt{R}}{(1-\nu^2)}$ | $\sqrt{R\delta}$ | $R$ is the indenter radius |
| conical | 2.0 | $\frac{2}{\pi}\frac{\tan\theta}{(1-\nu^2)}$ | $\delta \tan\theta$ | $\theta$ is the half-opening angle |

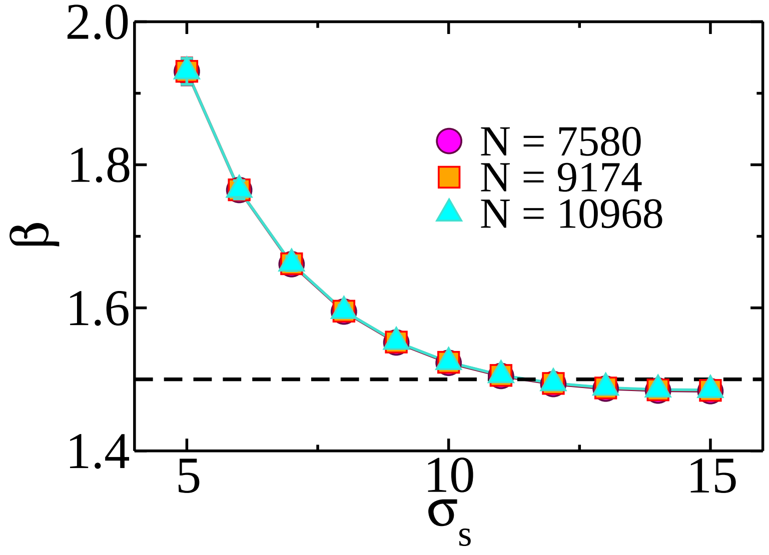


FIG. S1: The contact force $F$ between a spherical indenter and an elastic network, for height $H = 15\sigma$ and different numbers of particles $N$. $F$ is a power-law of the indentation depth, $F \propto \delta^{\beta}$, where the exponent $\beta$ depends on the indenter geometry [Ref. 28 in the main text]. This theory is based on the assumption that the sample is an elastic continuum half-space and the sample deformation is within the linear elastic regime. For conical, spherical and flat indenters, $\beta$ is given by 2, 3/2 and 1, respectively. For large $\sigma_s$, the sample experiences a force compatible with a flat indenter whereas the exponent of $\delta$ approaches the unity, while for small $\sigma_s$, the sample experiences a force compatible with a conical indenter and the exponent approaches 2. In our model, we find that $\sigma_s = 11\sigma$ is an intermediate value that recovers the exponent 3/2 for spherical indenters.

leaving to

$$f_l(t) = a_1 t^{3/2} + a_2\sqrt{t} + a_3\, erf\left(\sqrt{\frac{t}{\tau}}\right) e^{-t/\tau}, \qquad t \leq \tau_l, \tag{10}$$

$$f_d(t) = a_4 + a_5 e^{-(t-\tau_l)/\tau} + a_6 e^{-t/\tau}, \qquad t \geq \tau_l, \tag{11}$$

where the constants are given by

$$a_1 = \frac{E_\infty}{\tau_l^{3/2}}, \tag{12}$$

$$a_2 = \frac{3}{2}\frac{\tau}{\tau_l^{3/2}} E_0, \tag{13}$$

$$a_3 = -\frac{3}{4}\sqrt{\pi} E_0 \left(\frac{\tau}{\tau_l}\right)^{3/2}, \tag{14}$$

$$a_4 = E_\infty, \tag{15}$$

$$a_5 = \frac{3}{2}\frac{\tau}{\tau_l} E_0, \tag{16}$$

$$a_6 = a_3\, erf\left(\sqrt{\frac{\tau_l}{\tau}}\right). \tag{17}$$

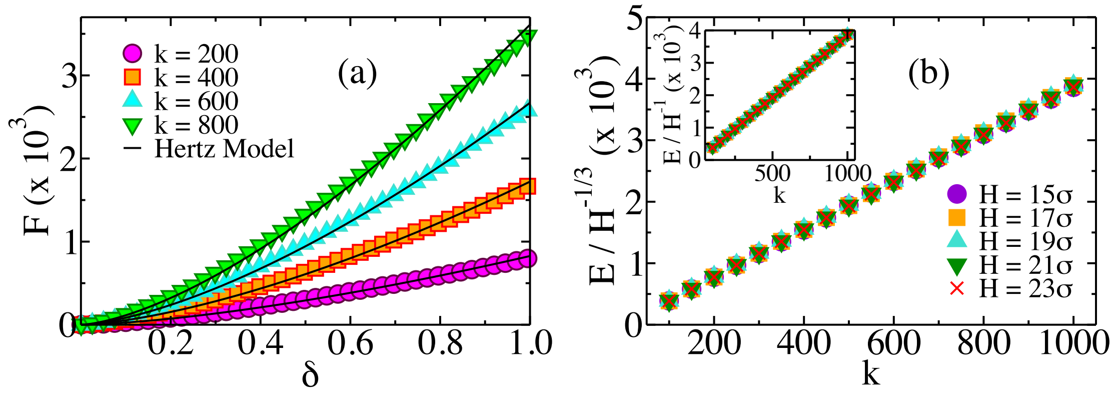


FIG. S2: (a) The contact force, $F$, probed by a spherical indenter as a function of the indentation depth, $\delta$, in homogeneous elastic networks for different value of $k$ and $H = 15\sigma$. We compute the elastic modulus $E$ by fitting our numerical data with the Hertz model (solid lines), shown in Eq. (3) in the main text, in different elastic networks. (b) As expected for homogeneous materials, $E$ displays a linear behavior with $k$. Moreover, $E$ is proportional to the sample height in the form $E \propto H^{-\zeta}$, where $\zeta$ depends on the indenter geometry. Spherical and flat indenters, for instance, give $\zeta = 1/3$ (main graph) and 1 (*inset plot*), respectively.

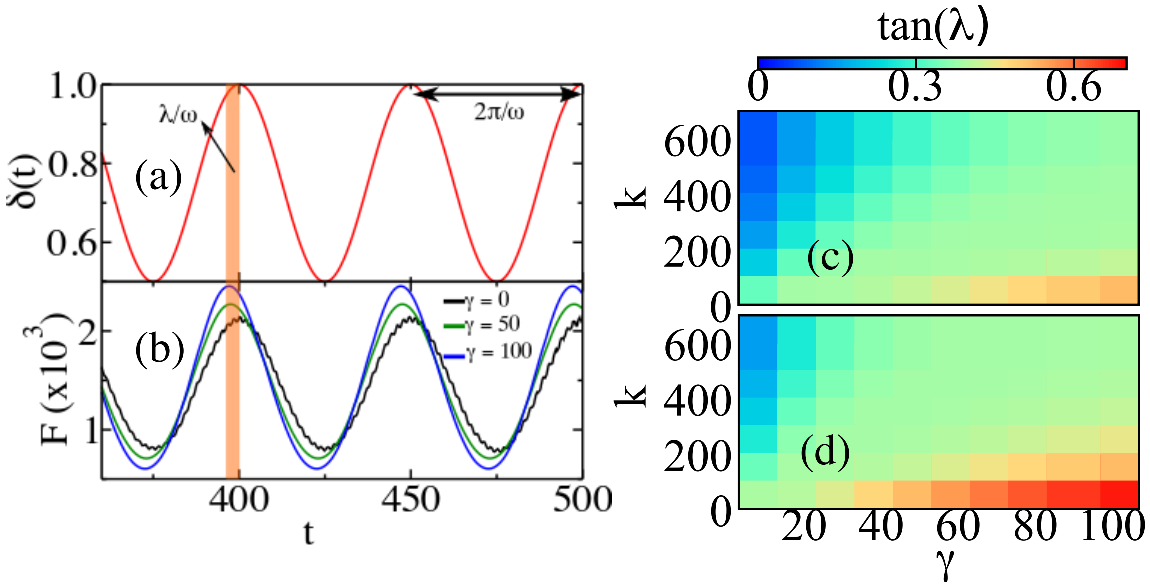


FIG. S3: Oscillatory experiments in homogeneous viscoelastic networks. A sinusoidal indentation, $\delta$, shown in (a) is applied to the network for $k = 500$ and different values of $\gamma$. Corresponding response forces, $F$, are shown in (b). The orange dashed lines highlight the phase lag, $\lambda$, between $F$ and $\delta$, which depends on viscoelastic properties. We also show color maps of $\tan(\lambda)$ for different values of $k$ and $\gamma$ for $\omega = 0.02$, in (c), and for $\omega = 0.04$, in (d).
